# Supplementary material for: Spatial anisotropy and heterogeneity in contractility and adhesion distribution may contribute to cell steering during migration
Source: arXiv:1310.7206 source file (2013-10-27)
Supplement: Supplementary file 1 [file supplementary.pdf]

**Spatial anisotropy and heterogeneity in contractility and adhesion distribution may contribute to cell steering during migration**

Soumya S S, Subodh Kolwankar, Edna George, Santanu K. Basu, Shamik Sen, and Mandar M. Inamdar

## SUPPLEMENTARY INFORMATION

## S1. Trypsin induced de-adhesion of L929 fibroblasts

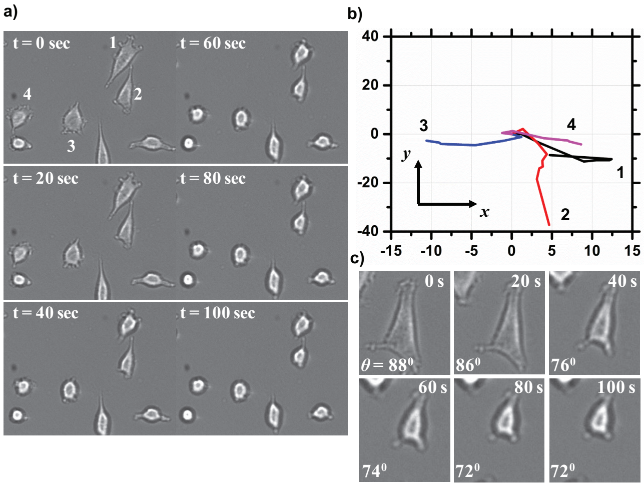


FIG. S1. (Color online) Trypsin induced de-adhesion of L929 fibroblasts. (a) Sequence of time-lapse images of L929 fibroblasts rounding up upon addition of trypsin. (b) Quantification of translation of L929 cells during de-adhesion. (c) Quantification of rotation of L929 cells during de-adhesion.

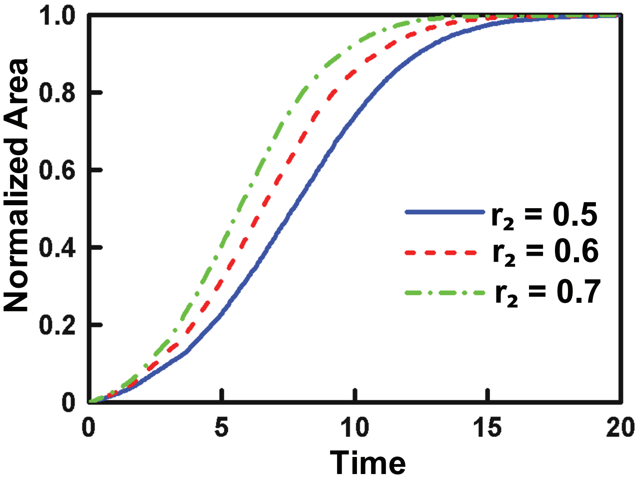


FIG. S2. (Color online) S-shaped de-adhesion curve for different bond cutting rates, $r_2$ for radially symmetric bond distribution $\rho_0 = 9r^4$; $r_1 = 50, r_3 = 0.1$

## S2. Derivation of equation of motion of the system

For a 2-D plane stress formulation in $\bar{x}$-$\bar{y}$ co-ordinate system, the strain-displacement relations are given by

$$\epsilon_{\bar{x}\bar{x}} = \frac{\partial \bar{u}}{\partial \bar{x}}, \tag{S1}$$

$$\epsilon_{\bar{y}\bar{y}} = \frac{\partial \bar{v}}{\partial \bar{y}}, \tag{S2}$$

$$\epsilon_{\bar{x}\bar{y}} = \frac{1}{2}\left(\frac{\partial \bar{u}}{\partial \bar{y}} + \frac{\partial \bar{v}}{\partial \bar{x}}\right), \tag{S3}$$

where $\bar{u}$ and $\bar{v}$ are the displacement components in $\bar{x}$ and $\bar{y}$ direction. The stress-strain relationship for a Kelvin-Voigt viscoelastic material[1,2] at any time $\bar{t}$ can be written as follows:

$$\sigma_{\bar{x}\bar{x}} = \frac{E_c}{(1-\nu^2)}\left(\epsilon_{\bar{x}\bar{x}} + \nu\epsilon_{\bar{y}\bar{y}}\right) + \frac{G_c}{(1-\nu^2)}\frac{\partial}{\partial \bar{t}}\left(\epsilon_{\bar{x}\bar{x}} + \nu\epsilon_{\bar{y}\bar{y}}\right), \tag{S4}$$

$$\sigma_{\bar{y}\bar{y}} = \frac{E_c}{(1-\nu^2)}\left(\nu\epsilon_{\bar{x}\bar{x}} + \epsilon_{\bar{y}\bar{y}}\right) + \frac{G_c}{(1-\nu^2)}\frac{\partial}{\partial \bar{t}}\left(\nu\epsilon_{\bar{x}\bar{x}} + \epsilon_{\bar{y}\bar{y}}\right), \tag{S5}$$

$$\tau_{\bar{x}\bar{y}} = \frac{E_c\epsilon_{\bar{x}\bar{y}}}{(1+\nu)} + \frac{G_c}{(1+\nu)}\frac{\partial \epsilon_{\bar{x}\bar{y}}}{\partial \bar{t}}, \tag{S6}$$

where $E_c$ and $G_c$ are the elastic and viscous modulus of the material.

The equations of equilibrium of the system can be written as

$$h_c\nabla.\boldsymbol{\sigma} + \boldsymbol{F} = 0. \tag{S7}$$

where $h_c$ is the average height of the cell and $\boldsymbol{F}$ is the surface traction (force/area) in the $\bar{x} - \bar{y}$ plane on the cell. Under plane stress condition, equilibrium equations of the system reduce to

$$\frac{\partial \sigma_{\bar{x}\bar{x}}}{\partial \bar{x}} + \frac{\partial \tau_{\bar{x}\bar{y}}}{\partial \bar{y}} + \frac{F_{\bar{x}}}{h_c} = 0, \tag{S8}$$

$$\frac{\partial \tau_{\bar{x}\bar{y}}}{\partial \bar{x}} + \frac{\partial \sigma_{\bar{y}\bar{y}}}{\partial \bar{y}} + \frac{F_{\bar{y}}}{h_c} = 0, \tag{S9}$$

where $F_{\bar{x}}$ and $F_{\bar{y}}$ are tractions acting in $\bar{x}$ and $\bar{y}$ direction respectively.

To get a relation between the substrate displacement $\bar{\boldsymbol{u}}_{\boldsymbol{s}}$ and traction, we assume that the force $\boldsymbol{f}$, which is transmitted by a single cell-substrate bond, is distributed uniformly over a circle of size $d_b$, the diameter of the bond[3]. Further, assuming the substrate with Young's modulus $E_s$ to be of much greater thickness as compared to the lateral extent of the cell, we use standard expressions to obtain a relation of the form $\boldsymbol{f} \approx E_s d_b \bar{\boldsymbol{u}}_{\boldsymbol{s}}$, where $\bar{\boldsymbol{u}}_{\boldsymbol{s}}$

is the displacement of the center of the circle[4]. The stiffness contributed from a single bond is thus $E_s d_b$. To be more precise, if we also incorporate the intrinsic stiffness of the bond $k_b$ to be in series with the substrate then the *effective* stiffness per bond-substrate complex will be

$$k_s = \frac{1}{\frac{1}{E_s d_b} + \frac{1}{k_b}}.$$

Now, if $\bar{\rho}_0 (\bar{x}, \bar{y})$ is the density of bonds, the total traction would be $\boldsymbol{F} = \bar{\rho}_0 k_s \boldsymbol{u_s}$.

After non-dimensionlizing all length scales with $R_{\text{cell}}$, substituting values from Eq. S1–S6, and recognizing that, $\bar{\boldsymbol{u}}_{\boldsymbol{s}} = \begin{Bmatrix} \bar{u}_0 - \bar{u}_c \\ \bar{v}_0 - \bar{v}_c \end{Bmatrix}$ and Eq. S8 and S9 reduce to following non-dimensionalized form

$$\frac{1}{2(1+\nu)} \nabla^2 u_c + \frac{1}{2(1-\nu)} \frac{\partial}{\partial x} \left( \frac{\partial u_c}{\partial x} + \frac{\partial v_c}{\partial y} \right) + r_1 \rho_0 (x, y) (u_0 - u_c) = 0, \tag{S10}$$

$$\frac{1}{2(1+\nu)} \nabla^2 v_c + \frac{1}{2(1-\nu)} \frac{\partial}{\partial y} \left( \frac{\partial u_c}{\partial x} + \frac{\partial v_c}{\partial y} \right) + r_1 \rho_0 (x, y) (v_0 - v_c) = 0. \tag{S11}$$

where the non-dimensionalized parameter $r_1 = \frac{E_s d_b}{E_c h_c}$. Here $u_0(x, y)$ and $v_0(x, y)$ denote the initial displacement field applied to cell to induce prestress.

During de-adhesion stage, when trypsin is added, the bond cutting process begins and bond density starts decaying exponentially. To get the equation of motion of this system at any time $\bar{t}$, re-write equation S8 and S9 by substituting values from equation S1 - S6. Then we get

$$\frac{\partial}{\partial \bar{x}} \left( \frac{E_c}{(1-\nu^2)} (\epsilon_{\bar{x}\bar{x}} + \nu \epsilon_{\bar{y}\bar{y}}) + \frac{G_c}{(1-\nu^2)} \frac{\partial}{\partial \bar{t}} (\epsilon_{\bar{x}\bar{x}} + \nu \epsilon_{\bar{y}\bar{y}}) \right) + \frac{\partial}{\partial \bar{y}} \left( \frac{E_c \epsilon_{\bar{x}\bar{y}}}{(1+\nu)} + \frac{G_c}{(1+\nu)} \frac{\partial \epsilon_{\bar{x}\bar{y}}}{\partial \bar{t}} \right) + \frac{\bar{\rho}_0 (\bar{x}, \bar{y})}{h_c} \exp(-r\bar{t}) \left( k_s (\bar{u}_0 - \bar{u}) + G_s d_b \frac{\partial}{\partial \bar{t}} (\bar{u}_0 - \bar{u}) \right) = 0, \tag{S12}$$

$$\frac{\partial}{\partial \bar{x}} \left( \frac{E_c \epsilon_{\bar{x}\bar{y}}}{(1+\nu)} + \frac{G_c}{(1+\nu)} \frac{\partial \epsilon_{\bar{x}\bar{y}}}{\partial \bar{t}} \right) + \frac{\partial}{\partial \bar{y}} \left( \frac{E_c}{(1-\nu^2)} (\nu \epsilon_{\bar{x}\bar{x}} + \epsilon_{\bar{y}\bar{y}}) + \frac{G_c}{(1-\nu^2)} \frac{\partial}{\partial \bar{t}} (\nu \epsilon_{\bar{x}\bar{x}} + \epsilon_{\bar{y}\bar{y}}) \right) + \frac{\bar{\rho}_0 (\bar{x}, \bar{y})}{h_c} \exp(-r\bar{t}) \left( k_s (\bar{v}_0 - \bar{v}) + G_s d_b \frac{\partial}{\partial \bar{t}} (\bar{v}_0 - \bar{v}) \right) = 0. \tag{S13}$$

As earlier, in order to non-dimensionalize the time and length scales with and $\tau_o = \frac{G_c}{E_c}$ and $R_{\text{cell}}$ respectively, we introduce the following non-dimensional parameters, $r_1 = \frac{E_s d_b}{E_c h_c}$,

$r_3 = \frac{G_s d_b}{G_c h_c}$ (derivation is similar to that of $r_1$ ), $r_2 = r\tau_0$ , $t = \frac{\bar{t}}{\tau_o}$. Eq. S12 and Eq. S13 then give

$$\frac{1}{2(1+\nu)}\left(\nabla^2 u + \frac{\partial}{\partial t}\nabla^2 u\right) + \frac{1}{2(1-\nu)}\frac{\partial}{\partial x}\left(\frac{\partial u}{\partial x} + \frac{\partial v}{\partial y}\right) + \frac{1}{2(1-\nu)}\frac{\partial}{\partial t}\frac{\partial}{\partial x}\left(\frac{\partial u}{\partial x} + \frac{\partial v}{\partial y}\right) + \rho_0(x,y)\exp(-r_2 t)\left(r_1(u_0 - u) - r_3\frac{\partial u}{\partial t}\right) = 0, \tag{S14}$$

$$\frac{1}{2(1+\nu)}\left(\nabla^2 v + \frac{\partial}{\partial t}\nabla^2 v\right) + \frac{1}{2(1-\nu)}\frac{\partial}{\partial y}\left(\frac{\partial u}{\partial x} + \frac{\partial v}{\partial y}\right) + \frac{1}{2(1-\nu)}\frac{\partial}{\partial t}\frac{\partial}{\partial y}\left(\frac{\partial u}{\partial x} + \frac{\partial v}{\partial y}\right) + \rho_0(x,y)\exp(-r_2 t)\left(r_1(v_0 - v) - r_3\frac{\partial v}{\partial t}\right) = 0. \tag{S15}$$

It is to be noted that in Eq. S10, S11, S14 and S15, all the length and time parameters are dimensionless. (The convention followed for representing symbols is that a quantity with dimension of length or time is denoted with a $\bar{()}$ on top of it and any parameter without $\bar{()}$ denote the corresponding dimensionless quantities of original equation.)

To solve these equations in the PDE toolbox of *MATLAB* using finite element analysis, Eqs. S14 and S15 are re-written in a vector form as

$$\frac{\partial}{\partial t}\left(\boldsymbol{d_{11}}u + \boldsymbol{d_{12}}v - \nabla(\boldsymbol{c_{11}}\nabla u) - \nabla(\boldsymbol{c_{12}}\nabla v)\right) - \nabla(\boldsymbol{c_{11}}\nabla u) - \nabla(\boldsymbol{c_{12}}\nabla v) + \boldsymbol{a_{11}}u + \boldsymbol{a_{12}}v = f_1, \tag{S16}$$

$$\frac{\partial}{\partial t}\left(\boldsymbol{d_{21}}u + \boldsymbol{d_{22}}v - \nabla(\boldsymbol{c_{21}}\nabla u) - \nabla(\boldsymbol{c_{22}}\nabla v)\right) - \nabla(\boldsymbol{c_{21}}\nabla u) - \nabla(\boldsymbol{c_{22}}\nabla v) + \boldsymbol{a_{21}}u + \boldsymbol{a_{22}}v = f_2, \tag{S17}$$

or

$$\frac{\partial}{\partial t}\left(\boldsymbol{d}u - \nabla.(\boldsymbol{c}\nabla u)\right) - \nabla.(\boldsymbol{c}\nabla u) + \boldsymbol{a}u = \boldsymbol{f}. \tag{S18}$$

where $\boldsymbol{c} = \begin{bmatrix} \boldsymbol{c_{11}} & \boldsymbol{c_{12}} \\ \boldsymbol{c_{21}} & \boldsymbol{c_{22}} \end{bmatrix}$ is a $2\times2\times2\times2$ tensor, $\boldsymbol{a} = \begin{bmatrix} \boldsymbol{a_{11}} & \boldsymbol{a_{12}} \\ \boldsymbol{a_{21}} & \boldsymbol{a_{22}} \end{bmatrix}$, $\boldsymbol{d} = \begin{bmatrix} \boldsymbol{d_{11}} & \boldsymbol{d_{12}} \\ \boldsymbol{d_{21}} & \boldsymbol{d_{22}} \end{bmatrix}$ are $2\times2$ matrices, $u = \begin{Bmatrix} u \\ v \end{Bmatrix}$ and $\boldsymbol{f} = \begin{Bmatrix} f_1 \\ f_2 \end{Bmatrix}$ are $2\times1$ vectors.

The values of $c$, $a$, $d$ and $f$ are given as follows

$\boldsymbol{c_{11}} = \begin{bmatrix} \frac{1}{1-\nu^2} & 0 \\ 0 & \frac{1}{2(1+\nu)} \end{bmatrix}$, $\boldsymbol{c_{12}} = \begin{bmatrix} 0 & \frac{1}{4(1-\nu)} \\ \frac{1}{4(1-\nu)} & 0 \end{bmatrix}$, $\boldsymbol{c_{21}} = \begin{bmatrix} 0 & \frac{1}{4(1-\nu)} \\ \frac{1}{4(1-\nu)} & 0 \end{bmatrix}$ and $\boldsymbol{c_{22}} = \begin{bmatrix} \frac{1}{2(1+\nu)} & 0 \\ 0 & \frac{1}{1-\nu^2} \end{bmatrix}$

$\boldsymbol{a_{11}} = \boldsymbol{a_{22}} = r_1\rho_0(x,y)\exp(-r_2t),\ \boldsymbol{a_{12}} = \boldsymbol{a_{21}} = 0,$

$\boldsymbol{d_{11}} = \boldsymbol{d_{22}} = r_3\rho_0(x,y)\exp(-r_2t),\ \boldsymbol{d_{12}} = \boldsymbol{d_{21}} = 0,$

$\boldsymbol{f_1} = r_1u_0(x,y)\,\rho_0(x,y)\exp(-r_2t),\ \boldsymbol{f_2} = r_1v_0(x,y)\,\rho_0(x,y)\exp(-r_2t).$

## S3. Expression for bond distribution for concentrated distribution of bonds at points $i$, $ii$ and $iii$ as shown in Fig. 4 of the main paper

$$\rho_{0(i)} = \frac{1}{\sqrt{2\pi\sigma^2}} exp\left(\frac{-\left(x-\cos(0)\right)^2-\left(y-\cos(0)\right)^2}{2\sigma^2}\right), \tag{S19}$$

$$\rho_{0(ii)} = \frac{1}{\sqrt{2\pi\sigma^2}} exp\left(\frac{-\left(x-\cos(0+2\pi/3)\right)^2-\left(y-\sin(0+2\pi/3)\right)^2}{2\sigma^2}\right), \tag{S20}$$

$$\rho_{0(iii)} = \frac{1}{\sqrt{2\pi\sigma^2}} exp\left(\frac{-\left(x-\cos(0+4\pi/3)\right)^2-\left(y-\sin(0+4\pi/3)\right)^2}{2\sigma^2}\right). \tag{S21}$$

The bond distribution function as shown in Fig. 4A

$$\rho_0(x,y,t) = \left(\rho_{0(i)} + 0.01\rho_{0(ii)} + 0.0001\rho_{0(iii)}\right)\exp(-r_2t), \tag{S22}$$

The bond distribution function as shown in Fig. 4B

$$\rho_0(x,y,t) = \left(\rho_{0(i)} + 0.1\rho_{0(ii)} + 0.01\rho_{0(iii)}\right)\exp(-r_2t), \tag{S23}$$

The bond distribution function as shown in Fig. 4C

$$\rho_0(x,y,t) = \rho_{0(i)} + \left(0.1\rho_{0(ii)} + 0.01\rho_{0(iii)}\right)\exp(-r_2t). \tag{S24}$$

## REFERENCES


[1]A. D. Mesquita and H. B. Coda, Eng. Anal. Bond. Elem. **27**, 885 (2003).

[2]H. Karcher, J. Lammerding, H. Huang, R. T. Lee, R. D. Kamm, and M. R. Kaazempur-Mofrad, Biophys. J. **85**, 3336 (2003).

[3]S. Walcott and S. X. Sun, Proc. Natl. Acad. Sci. **107**, 7757 (2010).

[4]L. Landau, E. Lifshitz, A. Kosevitch, and L. Pitaevskiui, *Theory of Elasticity*, Course of theoretical physics (Butterworth-Heinemann, UK, 1986).
